# Supplementary material for: Optimizing Binary Decision Diagrams with MaxSAT for classification
Source: arXiv:2203.11386 source file (2022-03-21)
Supplement: Supplementary file 1 [file 1-appendix.tex]

\appendix
\section{Appendix 1: Comparing the Original \Sat{} Encoding with the Improved Version}

%This appendix shows the improvements in reducing the encoding size of \Sat{} model of learning optimal \Bdd{}s.
We evaluate the first \Sat{} model (\Bdd{1} as described in Section~\ref{sec:Sat-models}) and the improved version (\Bdd{2} described in the same section~\ref{sec:Sat-models}) in terms of encoding size.
Considering the scalability problem, we use the hold-out method to split training set and testing set for all datasets.
We choose $5$ different small splitting ratios $r=\{0.05, 0.1, 0.15, 0.2, 0.25\}$ to generate training set.
The remaining examples for each ratio are used as testing set.
This process is repeated $10$ times with different random seeds.
The optimisation problem that we consider is to find a \Bdd{} that classifies all training examples with the minimum depth. 
The approach we use is a simple linear search by solving the decision problem that asks to find a $\Bdd$ with a given depth $H$ (Problem $P_{{bdd}}(\trainset, \depth)$).
The initial depth used in the linear search $\depth_0$ is set to $7$.
The \Sat{} solver we use is Kissat~\cite{BiereFazekasFleuryHeisinger-SAT-Competition-2020-solvers}, the winner of \Sat{} competition 2020.
For each experiment, we set $20$ hours as the global timeout for \Sat{} solver. 

In Table \ref{tab:annex1_satbdd_diff}, we report the average results of instances where all the runs finished within the limited time. 
The column ``Acc'' stands for average testing accuracy in percent, 
``dopt'' stands for the optimal depth,
``E\_Size'' stands for the encoding size (number of literals in 10 thousands),
and ``Time'' stands for the runtime in seconds of the successful runs. The value ``N/A'' indicates the lack of result. Finally, the blue color is used to show the best values. 

\input{tables/Annex1_satbdd_diff}

Table \ref{tab:annex1_satbdd_diff} shows that, compared to \Bdd{1}, \Bdd{2} improves clearly the encoding size and the run time. 
This empirical observation {confirms}
%proved 
the complexity {evaluation} for \Bdd{1} and \Bdd{2} {given} in Section~\ref{sec:Sat-models}.
%The phenomenon of the existing slight differences in testing accuracy {between} \Bdd{1} and \Bdd{2} is normal as two optimal solutions of the optimisation problem could be found (i.e., \Bdd s with different feature orderings). 

\section{Appendix 2: The Experiments Related to the Heuristic \MaxSat-\Bdd{} Method}

This appendix presents the details of the {comparative} evaluation {of}
%between 
\cart{}, heuristic \MaxSat-\Bdd{}, and the original \MaxSat-\Bdd{} in prediction quality, model size, encoding size, and run time.
The protocol of the experiments is described in Section~\ref{sec:exp}.

Table~\ref{tab:annex2_cart_hmaxsatbdd_maxsatbdd} shows the detailed results. 
The column ``Opt'' stands for the percentage of the instances reporting optimality,
``Time'' stands for the run time of the \MaxSat\ solver.
The other columns are described in Section~\ref{sec:exp}.

From Table~\ref{tab:annex2_cart_hmaxsatbdd_maxsatbdd}, we can first observe
%at first 
{that} the prediction quality of the heuristic \MaxSat-\Bdd{} is competitive to \cart{}.
The two scatter plots in Figure~\ref{fig:annex2_combined} show this fact more clearly.
Although, \cart{} could almost always get better training accuracy than the heuristic \MaxSat-\Bdd{}, it seems slightly over-fitting when {the} depth grows.

Compared to the original \MaxSat-\Bdd{}, our heuristic approach obtains clear benefits in terms of encoding size.
The reduction in encoding size gives more possibility to
the heuristic approach to report optimality within limited time, however using a subset of features (thus a relaxed version of the problem).
The results in columns ``Opt'' and ``Time'' illustrate this fact.

\begin{figure}[h!]
    \centering
    \begin{minipage}{0.49\linewidth}
        \centering
        \includegraphics[width=\linewidth]{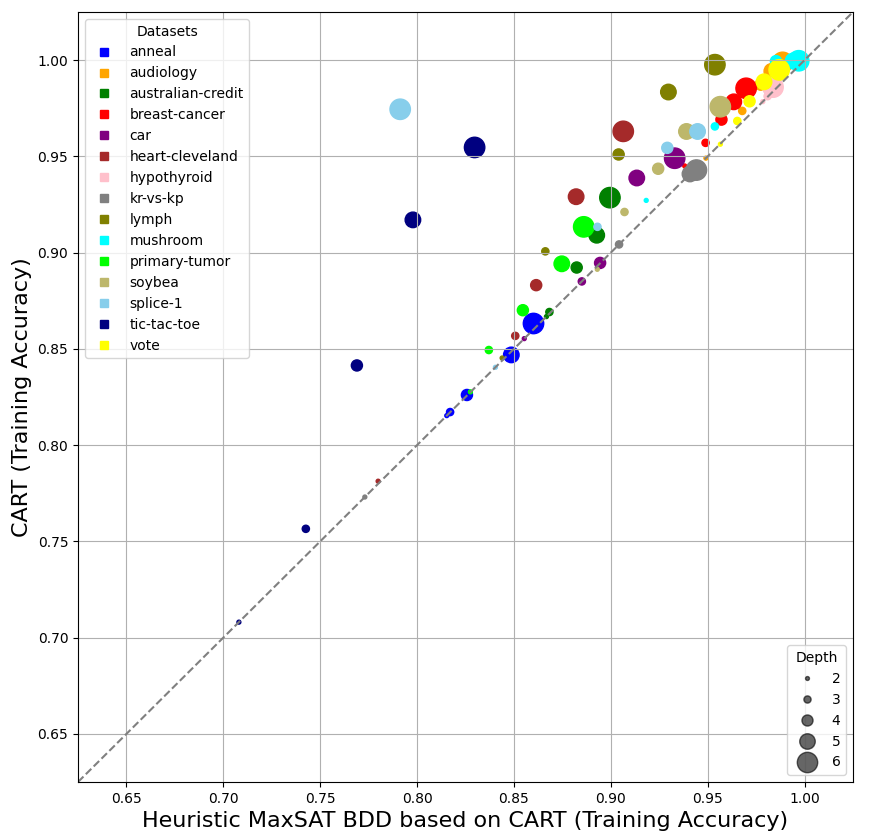}
    \end{minipage}\hfill
    \begin{minipage}{0.49\linewidth}
        \centering
        \includegraphics[width=\linewidth]{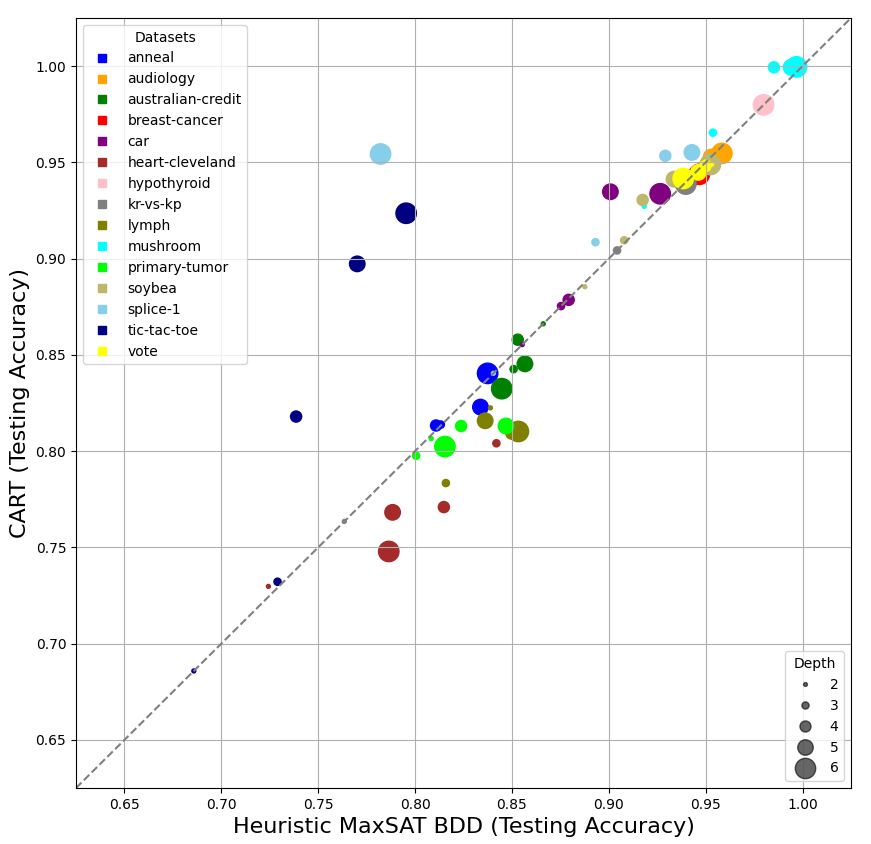}
    \end{minipage}
    \caption{\footnotesize{Comparison between \cart{} and Heuristic \MaxSat-\Bdd{} in training (the left one) and testing accuracy (the right one).}}
    \label{fig:annex2_combined}
\end{figure}

\input{tables/Annex2_cart_hmaxsatbdd_maxsatbdd}
